# Supplementary material for: A multiphase cubic MARS method for fourth- and higher-order interface tracking of two or more materials with arbitrary topology and geometry
Source: arXiv:2506.11897 source file (2026-04-03)
Supplement: Supplementary file 1 [file appendix_algorithms.tex]

\subsection{Enforcing $r_b>1$
  % the $(r_{\Tiny},h_L)$-regularity
  for not-a-knot splines}
\label{sec:NAK-r_tiny-h_l}

\begin{figure}
  \centering
  \subfigure[$\|p_1 - p_0\|_2 > \|p_2 - p_1\|_2$ implies $r_b< 1$]{
    \includestandalone[width=0.3\linewidth]{{\TIKZDIR}adjustEndsInit}
    \label{fig:adjustEndsInit}
  }
  \hfill
  \subfigure[insert a new marker between $p_0$ and $p_1$]{
    \includestandalone[width=0.28\linewidth]{{\TIKZDIR}adjustEnds1}
    \label{fig:adjustEnds1}
  }
  \hfill
  \subfigure[insert multiple new markers between $p_0$ and $p_1$]{
    %[$\|p_1 - q_1\|_2 > h_L$]{
    \includestandalone[width=0.28\linewidth]{{\TIKZDIR}adjustEnds2}
    \label{fig:adjustEnds2}
  }
  \caption{Algorithm~\ref{alg:adjustEnds}
    % in the $(r,h)$-regularity
    enforces $r_b>1$
    for the image of the breakpoint sequence
    of a not-a-knot spline $\mathbf{s}^{n}$
    under the discrete flow map $\varphi_{t_n}^k$. 
    In subplot (a),
    the three knots at the starting end $p_0$
    of $\varphi_{t_n}^k(\mathbf{s}^{n})$
    cause $r_b< 1$, where $p_0=S_{\varphi}(l_0)$, 
    $p_1=S_{\varphi}(l_1)$,
    and $S_{\varphi}:[l_0,l_1]\to\mathbb{R}^2$
    is given by $S_{\varphi}:=\varphi_{t_n}^k\circ\mathbf{s}^n$.
    As shown in Step (ARMS-4b) of Definition \ref{def:ARMS}, 
    this undesirable situation is fixed
    by first ensuring that the chordal length $\|p_0-p_1\|_2$
    is greater than $(1+r_b^{\ast})r_{\Tiny}h_L$, 
    then generating a sequence $\mathbf{q}$ of markers
    on the curve $S_{\varphi}([l_0,l_1])$, 
    and finally replacing $(p_0, p_1)$
    with $\mathbf{q}=(q_i)_{i=0}^M$. 
    The sequence $\mathbf{q}$ contains
    only three points if
    the new marker $q_1$ satisfies $\|p_1 - q_1\|_2 \leq h_L$; 
    see subplot (b) and lines~4--5 in Algorithm~\ref{alg:adjustEnds}.
    Otherwise $\mathbf{q}$ has more than three markers; 
    see subplot (c) and lines~6--9 in Algorithm~\ref{alg:adjustEnds}.
    % Subplot (a) is covered in Step (ARMS-4b)
    % in Definition \ref{def:ARMS}. 
    % The marker refinement between $p_0$ and $p_1$ 
    % in Algorithm~\ref{alg:adjustEnds}.
  }
  \label{fig:adjustEnds}
\end{figure}

% As the basis of the numerical analysis in Sec.~\ref{sec:analysis}, 
%  the $(r_{\Tiny},h_L)$-regularity of interface markers
%  is rigorously enforced
%  as a \emph{representation invariant} at each time step.

% The approximating spline set $S_{CT}$ in 
%  Definition~\ref{def:setOfFittedSplines} contains 
%  both periodic splines and not-a-knot splines. 

% To address the accuracy deterioration in 
% not-a-knot splines, we propose
% Algorithm~\ref{alg:adjustEnds} incorporating the
% ARMS strategy. The objective of Algorithm~\ref{alg:adjustEnds}
% is to ensure a lower bound $r_b^{\ast} > 1$ for $r_b$.

\begin{algorithm}[t]
  % \small
  \caption{: $\mathbf{q}$ = \texttt{adjustEnds}
    ($l_0, l_1$, $S_\varphi$, $r_{\Tiny}$, $h_L$, $r_b^{\ast}$)}
  % \hfill // partition $E$ into trails and circuits}
  \begin{algorithmic}[1]
    \REQUIRE An interval $[l_0, l_1]$;
    \\ \hspace{.6cm}
    a function $S_\varphi: [l_0, l_1] \rightarrow \mathbb{R}^2$;
    \\ \hspace{.6cm}
    the regularity parameters $(r_{\Tiny}, h_L)$;
    \\  \hspace{0.6cm}
    a desired lower bound $r_b^{\ast}$ of $r_b$ in (\ref{eq:rb}).
    \hspace{2cm} // we recommend $r_b^{\ast}=\frac{3}{2}$. 
    % $r_b^{\ast}, r_{\Tiny},$ and $h_L$
    % Parameters  $0 \le l_0 < l_1 \le L$,
    % a continuous bijective mapping 
    % $S_\varphi: [l_0, l_1] \rightarrow \mathbb{R}^2$, 
    % constants $r_b^{\ast}, r_{\Tiny},$ and $h_L$
    \ENSURE A marker sequence $\mathbf{q} := (q_i)_{i = 0}^M$. 
    \PreConditions 
    \hspace{0.03cm}
    (a) $l_1> l_0\ge 0$,
    $r_b^{\ast}\in \left(1, \frac{1}{2 r_{\Tiny}}\right)$, 
    $r_{\Tiny}\in \left(0, 
    \min(\frac{1}{6}, \frac{1}{2r_b^{\ast}}) \right)$;
    \\ \hspace{2.05cm}
    (b) $p_0 := S_\varphi(l_0)$ and $p_1 := S_\varphi(l_1)$
    satisfy $\|p_1 - p_0\|_2 > (1+r_b^{\ast})r_{\Tiny}h_L$; 
    \\ \hspace{2.05cm}
    (c) $S_\varphi$ is a continuous bijection.
    % Markers $(p_0, p_1, p_2)$ maintain 
    % parametric monotonicity on curve $S$

    \PostConditions
    (a)  $M\ge 2$ and
    % The corresponding parameters of 
    % generated sequence $\mathbf{q}$ on $S_{\varphi}$ maintain 
    % parametric strict monotonicity 
    $\forall i=0,\ldots, M-1$,
    $S_\varphi^{-1}(q_i) < S_\varphi^{-1}(q_{i+1})$; 
    % \hspace{2.3cm}
    \\ \hspace{2.05cm}
    (b) $q_0=p_0$; $q_{M}=p_1$; 
    $\forall i=1,\ldots, M-1$,\ 
    $q_i\in \{S_\varphi(l): \ l \in [l_0, l_1]\}$; 
    \\ \hspace{2.05cm}
    (c) $\mathbf{q}$ is $(r_{\Tiny}, h_L)$-regular
    as in Definition \ref{def:regularityCondition}; 
    \\ \hspace{2.05cm}
    (d) % The first three points of $\mathbf{q}$ satisfy 
    $r_b^{\ast}\|q_1 - q_0\|_2 \le \|q_2 - q_1\|_2$. 
    
    \STATE Initialize $\mathbf{q} \gets \emptyset$
    % \IF {$\|p_1 - p_0\|_2 \le \|p_2 - p_1\|_2$} 
    % \STATE $\mathbf{q} \gets (p_0, p_1, p_2)$
    % \RETURN 
    % \ENDIF
    \STATE Initialize $p_0 \gets S_\varphi(l_0); p_1 \gets S_\varphi(l_1); i \gets 0$

    % \STATE $q_0 \gets p_0$; $q_1 \gets p_1$
    % \IF {$\|p_1 - p_0\|_2 \le 2r_{\Tiny}h_L$}
    % \STATE $p_1 \gets p_2$;
    %        $l_1 \gets l_2$  \hfill
    %        // ensure $\|p_1 - p_0\|_2 > 2r_{\Tiny}h_L$
    % \ENDIF
    \STATE $q_i \gets p_0; \mathbf{q} \gets (q_i); i \gets i + 1$ \hfill
    // insert $p_0$ to $\mathbf{q}$ as $q_0$
    \Comment  // locate $q_1$ between $p_0$ and $p_1$
    \STATE $l \gets \texttt{BisectionSearch}\left(l_0, l_1, r_{\Tiny}h_L, 
    \min\left(\frac{1}{2r_b^{\ast}}h_L, 
          \frac{1}{1+r_b^{\ast}}
          \|p_1 - p_0\|_2\right), S_\varphi\right)$ 
    \STATE $q_i \gets S_\varphi(l); \mathbf{q} \gets (\mathbf{q}, q_i); 
    i \gets i + 1$ \hfill
    % // insert $q_1$ to $\mathbf{q}$
    \Comment  // ensure maximum chordal length $ \le h_L$
    \WHILE{${\|p_1 - q_{i - 1}\|_2} > h_L$}
    % \STATE $l_l \gets l$; $l_r \gets l_1$; $l \gets \frac{l_l + l_r}{2}$; $q \gets \varphi_{t_n}^k(\mathbf{s}^n(l))$
    \Comment // locate $q_i$ between $q_{i-1}$ and $p_1$
    \STATE $l \gets \texttt{BisectionSearch}\left(l, l_1, \frac{1}{2}h_L, 
    \min\left(h_L, \frac{1}{2}\|p_1 - q_{i - 1}\|_2\right), \left.S_\varphi\right|_{[l,l_1]}\right)$ 
    \STATE $q_i \gets S_\varphi(l);\mathbf{q} \gets (\mathbf{q}, q_i); i \gets i + 1$ 
    % \hfill // insert $q_i$ to $\mathbf{q}$
    \ENDWHILE

    \STATE $q_i \gets p_1; \mathbf{q} \gets (\mathbf{q}, q_i)$\hfill
    // ensure that $p_1$ is the last marker of $\mathbf{q}$
    % \IF{$p_1 \not= p_2$} 
    % \STATE $\mathbf{q} \gets (\mathbf{q}, p_2)$
    % \ENDIF
    % \RETURN $\mathbf{q}$
\end{algorithmic}

\vspace{3mm} % 添加间距分隔主算法和子函数
\begin{algorithmic}[1]
\makeatletter
  \setcounter{ALC@line}{10} 
\makeatother
    \STATE 
    \textbf{subroutine}: $l$ = \texttt{BisectionSearch}($l_l, l_r, \text{low}, \text{high}, S_\varphi$) 
    \REQUIRE An interval $[l_l, l_r]$; 
    a target interval $[\text{low}, \text{high}]$; 
    a function $S_\varphi:[l_l,l_r]\to \mathbb{R}^2$. 
    \ENSURE A parameter $l$.
    \PreConditions \hspace{0.3mm}
    (a) $S_\varphi$ is continuous; \ 
    (b) $0\le \text{low} < \text{high}\le
    \|S_\varphi(l_r) - S_\varphi(l_l)\|_2$. 
    % $[\text{low}, \text{high}] \subset 
    % \left[0, \|S_\varphi(l_r) - S_\varphi(l_l)\|_2 \right]$;    
%    \\ \hspace{2.22cm}
    
    \PostConditions
    (a) $l\in (l_l,l_r)$; \hspace{9.0mm}
%    \\ \hspace{2.22cm}
    (b) $\|S_\varphi(l) - S_\varphi(l_l)\|_2 \in [\text{low}, \text{high}]$. 
%    where $d_S(l):=\|S_\varphi(l) - S_\varphi(l_l)\|_2$.
% \Function{BisectionSearch}{$l_l, l_r, low, \text{high}, S_\varphi$}
    \STATE $p_l \gets S_\varphi(l_l)$;\ $l \gets \frac{l_l + l_r}{2}$
    % $; p_r \gets S_\varphi(l_r)$
    % \STATE 
    % ; p_m \gets S_\varphi(l)$
    \WHILE{$\|S_\varphi(l )- p_l\|_2 \not\in [\text{low}, \text{high}]$}
        \IF{$\|S_\varphi(l) - p_l\|_2 < \text{low}$}
            \STATE $l_l \gets l$
        \ELSE 
            \STATE $l_r \gets l$
        \ENDIF
        \STATE $l \gets \frac{l_l + l_r}{2}$ %; $p_m \gets S_\varphi(l)$
    \ENDWHILE
    % \RETURN $l$
% \endFunction
% \Statex % 空行(可选,用于分隔)
  \end{algorithmic}
  \label{alg:adjustEnds}
\end{algorithm}

By Theorems \ref{thm:notaKnotSplineErrorEstimates} 
 and \ref{thm:periodicSplineErrorEstimates}, 
 not-a-knot splines are fundamentally different
 from periodic splines
 in that their interpolation errors
 depend on $r_b$ in (\ref{eq:rb})
 and are thus affected by the ratio of distances
 between the three markers at any of the two ends 
 of the interpolation range.
Even if the breakpoint sequence $(X_i)_{i=0}^N$ of
 a not-a-knot spline $\mathbf{s}^n$ %$: [0,L^n]\to \mathbb{R}^2$
 satisfies both the condition $r_b>1$ and the $(r,h)$-regularity, 
 none of these conditions may hold for
 the image sequence $(p_i)_{i=0}^N$ where
 $ p_i= \varphi_{t_n}^k(X_i)$ for each $i$;
 % of $(X_i)$ the breakpoint sequence of $\mathbf{s}^n$
 % under the discrete flow map $\varphi_{t_n}^k$;
 see Fig.~\ref{fig:adjustEnds}(a) for an example
 of $r_b$ becoming less than 1 at the left end of $(p_i)_{i=0}^N$. 
Consequently, a small value of $r_b$
 may lead to severe accuracy deteriorations.
Since the user-specified value of $r_{\Tiny}$
 may be much less than 1,
 $(r_{\Tiny},h_L)$-regularity does not imply $r_b>1$. 
Indeed, these two conditions are independent to each other.
% This is the reason why Definition \ref{def:regularityCondition-NAK}
%  differs from Definition \ref{def:regularityCondition-P}.

Given an interval $[l_0, l_1]$,
 a continuous bijection
 $S_\varphi: [l_0, l_1] \rightarrow \mathbb{R}^2$ 
 satisfying $p_0=S_{\varphi}(l_0)$ and $p_1=S_{\varphi}(l_1)$, 
 the regularity parameters $(r_{\Tiny}, h_L)$, 
 and a lower bound $r_b^{\ast}>1$, % of $r_b$ in (\ref{eq:rb}), 
 %the pre-conditions (a,b,c),
 Algorithm~\ref{alg:adjustEnds} outputs 
 a sequence $\mathbf{q}=(q_i)_{i=0}^M$ of breakpoints
 on the curve segment $S_{\varphi}([l_0,l_1])$
 so that $(q_0, q_1, \ldots, q_M, p_2, \ldots)$
 constitutes the left end of the $(r_{\Tiny}, h_L)$-regular sequence
 for fitting a not-a-knot spline at time $t_{n+1}$.
In particular, post-condition (d)
 guarantees $r_b>r_b^{\ast}$.
 % The right end of the desired sequence
%  can be generated by calling Algorithm~\ref{alg:adjustEnds}

To meet the mutual dependence
 between the upper bounds of $r_b^{\ast}$ and $r_{\Tiny}$
 in pre-condition (a),
 we recommend choosing $r_b^{\ast}=\frac{3}{2}$.
To satisfy pre-condition (b),
 one might have to repeatedly remove $p_1$ until
 the updated marker sequence satisfies
 $\|p_1 - p_0\|_2 > (1+r_b^{\ast})r_{\Tiny}h_L$.
% before the determination of $l_1$ and $S_{\varphi}$. 
Since $\varphi_{t_n}^k$ is a homeomorphism
 and any $\mathbf{s}^n\in S_{CT}^n$ is $\mathcal{C}^2$, 
pre-condition (c) always holds
 for $S_{\varphi}=\varphi_{t_n}^k\circ\mathbf{s}^n$. 

% if we don't handle the three breakpoints near 
% the endpoints, then $r_b$ might be very close to $r$ 
% in Definition~\ref{def:regularityCondition}.
% Hence the error term in (\ref{eq:notaKnotSplineErrorEstimates})
% degrades from $O(h_L^4)$ to $O\left(
% \frac{h_L^4}{r}\right)$, which results in accuracy deterioration
% for not-a-knot splines when $r$ is small 
% (a scenario frequently observed in
% the numerical experiments, see Sec.~\ref{sec:tests}).

At the core of Algorithm \ref{alg:adjustEnds}
 is the subroutine \texttt{BisectionSearch}
 for finding a parameter $l\in [l_l, l_r]$
 so that the distance $\|S_\varphi(l) - S_\varphi(l_l)\|_2$
 is within the given range $[\text{low}, \text{high}]$.
The existence of such a parameter
 is guaranteed by the intermediate value theorem.
As shown in Fig.~\ref{fig:adjustEnds}(b),
 we set $q_1=S_{\varphi}(l)$
 after locating a parameter $l\in [l_0,l_1]$ of $\mathbf{s}^n$.
If $\|q_1-p_1\|_2>h_L$,
 multiple markers are inserted between
 $p_0$ and $p_1$; see Fig.~\ref{fig:adjustEnds}(c). 

The correctness proof of Algorithm~\ref{alg:adjustEnds}
 is given in Appendix~\ref{sec:proofAlgorithms}.

%  \texttt{BisectionSearch} and 
% As a \emph{representation invariant}
%  enforced throughout IT,
%  the $(r_{\Tiny},h_L)$-regularity
%  also facilitates the numerical analysis in
%  Sec.~\ref{sec:analysis}. 

\begin{lem}
  \label{lem:algorithmBisectionSearch}
  Provided that its pre-conditions hold, 
  the \texttt{BisectionSearch} subroutine in Algorithm~\ref{alg:adjustEnds}
  stops and its post-conditions hold.
\end{lem}
\begin{proof}
  Define a function $d_S(l):=\|S_\varphi(l) - S_\varphi(l_l)\|_2$
  where $l_l$ is the left end of the input interval.
  Since $S_{\varphi}$ is continuous,
  $d_S$ is also continuous.

  Denote respectively by $l_l^{(0)}$ and $l_r^{(0)}$
  the values of $l_l$ and $l_r$ at line 12. 
  Denote respectively by $l_l^{(n)}$ and $l_r^{(n)}$
  the values of $l_l$ and $l_r$ at line 19  
  in the $n$th iteration
  of the while loop. % between lines~13--20.
  Pre-condition~(b) yields
  $d_S(l_l^{(0)}) \leq \text{low} < \text{high} \leq d_S(l_r^{(0)})$.
  % $=\|S_\varphi(l_r) - S_\varphi(l_l)\|_2$.

  Suppose the while loop never terminates. 
  Then, for each iteration,
  the conditionals at lines 13,14,16
  and the assignments at lines 15,17,19 imply
  \begin{displaymath}
    \begin{array}{l}
    \forall n=1,2,\ldots, \quad
    d_S\left(l_l^{(n)}\right) < \text{low};\
     d_S\left(l_r^{(n)}\right) > \text{high};\quad
    l_r^{(n)} - l_l^{(n)} = 
    \frac{1}{2}\left(l_r^{(n-1)} - l_l^{(n-1)}\right).
    \end{array}
  \end{displaymath}
  Consequently, for the constant $\delta := \text{high} - \text{low} > 0$,
  we have 
  \begin{displaymath}
    \begin{array}{l}
    \forall \epsilon > 0, \  \exists N > 0, 
    \text{ s.t. } \forall n > N, \quad 
    \left|l_r^{(n)} - l_l^{(n)}\right| < \epsilon; \ 
    \left|d_S\left(l_r^{(n)}\right) - d_S\left(l_l^{(n)}\right)\right| 
    > \delta,
    \end{array}
  \end{displaymath}
  which contradicts the continuity of $d_S$.
  Hence, the while loop must exit with
  post-condition (b) satisfied. 
  Post-condition~(a) also holds because 
  the assignments at lines 12, 15, 17, 19
  never create any value of $l$ outside $[l_l, l_r]$. \qed
  % and the intermediate value theorem 
  % imply that for any $v\in[\text{low}, \text{high}]$,
  % there exists $l_v\in [l_l,l_r]$
  % such that $d_S(l_v)=v$.
  % Since $\text{low}<\text{high}$, 
  % the interval $[\text{low}, \text{high}]$
  % has a finite width.
  % Then the while loop in lines 14--21 must exist
  % because for each iteration
  % the remaining range of interval for the search of $l$ is halved. 
\end{proof}

Note that, 
for each invocation of \texttt{BisectionSearch}
in Algorithm \ref{alg:adjustEnds}, 
the function $d_S$ in the proof of Lemma \ref{lem:algorithmBisectionSearch}
is different.

\begin{lem}
  \label{lem:algorithmAdjustEnds}
  If its pre-conditions hold, 
  Algorithm~\ref{alg:adjustEnds} stops and
  its post-conditions hold.
\end{lem} 
\begin{proof}
  For the new marker $q_1$ inserted at lines 4--5, 
  pre-conditions (a,b) yield 
  \begin{displaymath}
    \begin{array}{l}
    0 < r_{\textup{tiny}}h_L <
    \min\left(\frac{1}{2r_b^{\ast}}h_L, 
    \frac{1}{1+r_b^{\ast}}\|p_1 - q_0\|_2\right) 
    < \|p_1 - q_0\|_2.
    \end{array}
  \end{displaymath}
  Thus pre-conditions of \texttt{BisectionSearch} at line 4 hold
  and, by Lemma \ref{lem:algorithmBisectionSearch}, 
  \texttt{BisectionSearch} must terminate
  with its post-conditions satisfied, i.e.,
  \begin{equation}
    \label{eq:binarySearch1-post}
    \begin{array}{l}
    r_{\text{tiny}}h_L \leq \|q_1 - q_0\|_2 \leq 
    \min\left(\frac{1}{2r_b^{\ast}}h_L, 
      \frac{1}{1+r_b^{\ast}} \|p_1 - p_0\|_2
    \right) < h_L, 
    \end{array}
  \end{equation}
  which further implies 
  \begin{equation}
    \label{eq:q1q0UpperBnd}
    \begin{array}{l}
    (1+r_b^{\ast})\|q_1 - q_0\|_2 \le \|p_1 - p_0\|_2
    \le (\|p_1 - q_1\|_2+\|q_1 - q_0\|_2),
    \end{array}
  \end{equation}
  where %the first inequality follows from (\ref{eq:binarySearch1})
  the second inequality follows from $q_0=p_0$  and the triangle inequality.
  
  If the loop in lines 6--9 is not entered,
  Algorithm \ref{alg:adjustEnds} terminates with $q_2=p_1$ at line 10.
  The first and the last terms in (\ref{eq:q1q0UpperBnd}) yield
  post-condition (d), i.e., 
  \begin{equation}
    \label{eq:proofAlg2-d}
    \begin{array}{l}
    r_b^{\ast}\|q_1 - q_0\|_2 \le \|q_2 - q_1\|_2.
    \end{array}
  \end{equation}
%  which gives $\|p - q_1\|_2,$
  Then we have
  \begin{equation}
    \label{eq:firstInsert}
    \begin{array}{l}
    r_{\text{tiny}}h_L < r_b^{\ast}\|q_1 - q_0\|_2 
    \le \|p_1 - q_1\|_2 \le h_L, 
    \end{array}
  \end{equation}
  where the first inequality follows from (\ref{eq:binarySearch1-post}) and
  $r_b^{\ast}>1$,
  the second from (\ref{eq:proofAlg2-d}) and $q_2=p_1$,
  and the last from the conditional in line 6 being false.
  Therefore, in this case of $M=2$,
  post-condition (c) follows from (\ref{eq:binarySearch1-post})
  and (\ref{eq:firstInsert}). 

  Otherwise, the loop in lines 6--9 is entered
  and each iteration satisfies 
  \begin{equation}
    \label{eq:binarySearch2-pre}
    \begin{array}{l}
    0 < \frac{1}{2}h_L 
    < \min\left(h_L, \frac{1}{2}\|p_1 - q_{i - 1}\|_2\right)
    \le h_L < \|p_1 - q_{i - 1}\|_2, 
    \end{array}
  \end{equation}
  where the second and the last inequalities follow from 
  the conditional in line 6 being true.
  By (\ref{eq:binarySearch2-pre}),
  pre-conditions of \texttt{BisectionSearch} hold 
  and then Lemma \ref{lem:algorithmBisectionSearch} gives
  \begin{equation}
    \label{eq:binarySearch2-post}
    \begin{array}{l}
    \frac{1}{2}h_L \leq \|q_i - q_{i - 1}\|_2 
    \le \min\left(h_L, \frac{1}{2}\|p_1 - q_{i - 1}\|_2\right). 
    \le h_L < \|p_1 - q_{i - 1}\|_2, 
    \end{array}
  \end{equation}
  Then $\|q_{M-1} - q_{M - 2}\|_2
  \le \frac{1}{2}\|p_1 - q_{M - 2}\|_2$
  and the triangle inequality imply 
  \begin{equation}
    \label{eq:post(d)-last}
    \begin{array}{l}
    \frac{1}{2}h_L \leq \|q_{M-1} - q_{M - 2}\|_2 
    \le \|p_1 - q_{M - 1}\|_2\le h_L.
    \end{array}
    %\le h_L < \|p_1 - q_{i - 1}\|_2, 
  \end{equation}
  To sum up for $M>2$,
  post-condition (c) follows
  from (\ref{eq:binarySearch2-post}) and (\ref{eq:post(d)-last}); 
  post-condition (d) also holds
  because (\ref{eq:binarySearch1-post}) gives 
  $r_b^{\ast}\|q_1 - q_0\|_2 \le \frac{1}{2}h_L$
  and (\ref{eq:binarySearch2-post}) yields
  $\frac{1}{2}h_L \leq \|q_2 - q_{1}\|_2 $.
  
  For the parameter $l_{q_1}$ satisfying
  $S_{\varphi}(l_{q_1})=q_1$, 
  the curve segment $S_{\varphi}([l_{q_1}, l_1])$
  has a finite arc length, 
  which, after each iteration in lines 7--8,
  is reduced at least by $\frac{1}{2}h_L$, cf. (\ref{eq:binarySearch2-post}).
  Hence the while loop in lines 6--9 must stop.
  
  Finally,
  the insertion order in lines 2, 3, 8, and 10 
  ensures the marker sequence $\mathbf{q}$ starts at $q_0=p_0$, ends
  at $q_M=p_1$, and the corresponding parameters on $S_{\varphi}$
  are strictly increasing.
  Thus post-condition (a) holds.
  Post-condition (b) also holds
  because, for any $i=0,1,\ldots,M$, 
  $q_i$ is always assigned as a function value of $S_{\varphi}$.  \qed
\end{proof}

%%% Local Variables: 
%%% mode: latex
%%% TeX-master: "../MARS-n2D"
%%% End: 

% LocalWords:  multiphase advecting substep advection isocontour MOF
% LocalWords:  substeps cellwise VOF Voronoi normals centroids
% LocalWords:  homeomorphic semianalytic
