# Supplementary material for: A multiphase cubic MARS method for fourth- and higher-order interface tracking of two or more materials with arbitrary topology and geometry
Source: arXiv:2506.11897 source file (2026-04-03)
Supplement: Supplementary file 2 [file appendix_splines.tex]

In this appendix,
 we show that it is numerically stable
 to interpolate closed curves and curve segments
 respectively by periodic and not-a-knot splines: 
 an ${O}(\epsilon)$ perturbation to a breakpoint
 causes an $O(\epsilon)$ error to the fitted spline. 
 % is guaranteed by 
 % Lemma~\ref{lem:splineLocality} and \ref{lem:splineStability}.

% \subsubsection{Perturbing breakpoints of periodic and
%   not-a-knot cubic splines}
% \label{sec:pert-breakp-peri}

We first establish a constants upper bound of $\|A^{-1}\|_1$
 by applying the Demko's Theorem
\begin{thm}[Demko \cite{demko1977}]
    \label{thm:demko}
    Let $A =(a_{i,j})$ be an $n \times n$ matrix. 
    Assume that there is a number $m$ such that $a_{i,j} = 0$ 
     if $|i-j| > m$ and that $\|A\|_q \le 1$ 
     and $\|A^{-1}\|_q \le \mu^{-1}$ for 
     some $1 \le q \le \infty$ and some $\mu > 0$. 
    Then, with $A^{-1} = (\alpha_{i,j})$, 
    there are numbers $K > 0$ and $r \in (0, 1)$ 
    depending only on $\mu$ and $m$ such that for all $i, j \in 
    \{1, 2, \cdots, n\}$, we have
    \begin{equation*}
        |\alpha_{i,j}| \le K r^{|i - j|}.
    \end{equation*}
\end{thm}

\begin{lem}
    \label{lem:inverseA-1Norm}
    For any given $f \in \mathcal{C}^2([a,b])$
    and breakpoint sequence $X_b$ over $[a,b]$ with 
    \mbox{$N \ge 5$}, 
    the matrix $A$ defined in \eqref{eq:miLinearSystem2} satisfies 
    $\|A^{-1}\|_1 < C$, where $C$ is a constant independent of $X_b$.
\end{lem}
\begin{proof}
    According to Lemma~\ref{lem:inverseA-inftyNorm},
     Theorem~\ref{thm:demko} with
     parameters $n = N+1$, $\mu = \frac{1}{18}$, $m = 2$, and $q = \infty$ demonstrates
     that the entries of the inverse matrix $A^{-1} = (\alpha_{i,j})$ 
     satisfy
    \begin{equation*}
      \begin{array}{rl}
        |\alpha_{i,j}| \le K r^{|i - j|} 
      \end{array}
    \end{equation*}
     for some constants $K > 0$ and $r \in (0, 1)$.
    Consequently, we can bound the 1-norm of the inverse matrix as follows
    \begin{equation*}
      \begin{array}{rl}
        \|A^{-1}\|_1 = \max_{1 \le j \le N + 1} \sum\nolimits_{i = 1}^{N+1} |\alpha_{i, j}| 
        &\le K \max_{1 \le j \le N + 1}  
        \left(\sum\nolimits_{i = 1}^{j} r^{j - i} + 
                    \sum\nolimits_{i = j+1}^{N+1} r^{i - j} \right)  \\
        &\le 2 K \sum\nolimits_{i = 0}^N r^{i} = \frac{2K(1 - r^{N+1})}{1 - r}
        < \frac{2K}{1 - r}.
      \end{array}
    \end{equation*}
    Thus, the proof is completed by choosing 
     the constant $C = \frac{2K}{1 - r}$, which is independent of 
     the breakpoint sequence $X_b$.
     \qed
\end{proof}

For a spline $S$, %$S: \mathcal{L}\rightarrow\mathbb{R}^2$, 
 denote by $\mathcal{L}:=[l_0,l_{N}]$
 the interval of the cumulative chordal length
 and $l_0, l_1, \ldots, l_{N}$ the knots 
 satisfying $\Delta l_i := l_{i+1} - l_i = O(h)$
 and \mbox{$S(l_{i+1}) - S(l_i) = \mathbf{O}(h)$}.
An ${O}(\epsilon)$ perturbation with $\epsilon\ll h$
 to knots of $S(l)$
 yields a new spline $\hat{S}: \mathcal{\hat{L}}\to \mathbb{R}^2$ 
 with $\mathcal{\hat{L}}:=[\hat{l}_0,\hat{l}_{N}]$
 and the new knots $\hat{l}_0, \hat{l}_1, \ldots, \hat{l}_{N}$ 
 satisfy 
 \begin{equation}
   \label{eq:S_perturb}
   \Delta \hat{l}_i := \hat{l}_{i+1} - \hat{l}_i = O(h);\ 
   \hat{S}(\hat{l}_i)-S(l_i) = \mathbf{O}(\epsilon);\ 
   % \\
   % \label{eq:dl_perturb}
   %\text{ and } 
   \Delta\hat{l}_i - \Delta l_i = O(\epsilon).
 \end{equation}
 
We also construct a bijection $\upsilon:\mathcal{L}\to\hat{\mathcal{L}}$
 that maps each $[l_i,l_{i+1}]$ to $[\hat{l}_i,\hat{l}_{i+1}]$, 
 \begin{equation}
   \label{eq:LTohatL}
   \begin{array}{rl}
     \hat{l}|_{[\hat{l}_i,\hat{l}_{i+1}]}
     =\upsilon|_{[l_i,l_{i+1}]}(l)
     =\frac{\Delta\hat{l}_i}{\Delta l_i}
     \left(l-l_i\right)+\hat{l}_i.
   \end{array}
 \end{equation}
 
\begin{lem}
\label{lem:splineLocality}
  Let $\{\mathbf{X}_i\}_{i=0}^N$ be an 
  $(r, h)$-regular sequence for periodic or not-a-knot splines.
  Perform an $O(\epsilon)$ perturbation 
  to a single breakpoint
  $\mathbf{X}_j$ for some $j=1,\ldots,N-1$,
  and denote by $S:\mathcal{L} \to \mathbb{R}^2$
  and $\hat{S}:\hat{\mathcal{L}} \to \mathbb{R}^2$ the 
  cubic splines before and after the perturbation, respectively.
  Then, we have
  \begin{equation*}
      \int_{l_0}^{l_{j-1}} \left\|S(l) - \hat{S}(\upsilon(l))\right\|_2
      \mathrm{d} l + \int_{l_{j+1}}^{l_{N}} \left\|S(l) -
      \hat{S}(\upsilon(l)) \right\|_2 \mathrm{d} l = O(\epsilon h),
  \end{equation*}
  where 
  % $\mathcal{L} := 
  % [l_0, l_{N}]$ is the interval of the cumulative chordal 
  % length and $l_0,\ldots,l_{N}$ the knots of $S$, 
  % $\hat{\mathcal{L}} := [\hat{l}_0, \hat{l}_{N}]$ and 
  % $\hat{l}_0,\ldots,\hat{l}_{N}$ denote that of $\hat{S}$. 
  the bijection $\upsilon$ maps each $[l_i,l_{i+1}]$
  to $[\hat{{l}_i},\hat{l}_{i+1}]$ as defined in (\ref{eq:LTohatL}).
\end{lem}
\begin{proof}
% The key lies in the strictly diagonal dominance 
% property of the linear system. 
We only prove the conclusion for not-a-knot cubic splines
since the case of periodic splines can be proven similarly.

The cumulative chordal length (\ref{eq:cumulativeChordalLength})
and the $(r, h)$-regularity yield
\begin{equation}
    \label{eq:LhatErr}
     \begin{aligned}
       \forall i\notin \{j-1,j\}, \quad  
       &\Delta \hat{l}_i -\Delta l_i =
         (\hat{l}_{i+1} - \hat{l}_{i})
         - (l_{i+1} - l_{i}) = 0,\\
       &\Delta \hat{l}_{j-1} -\Delta l_{j-1} =  
       (\hat{l}_{j} - \hat{l}_{j-1})
        - (l_{j} - l_{j-1}) = O(\epsilon),\\
       &\Delta \hat{l}_{j} -\Delta l_{j} =  
        (\hat{l}_{j+1} - \hat{l}_{j})
        - (l_{j+1} - l_{j}) = O(\epsilon),
     \end{aligned}
\end{equation}
and the bijection $\upsilon$ can be simplified as
\begin{equation}
\begin{aligned}
    \label{eq:bijectionofL}
    \forall i=0,\ldots, j-2, \quad  
    \upsilon|_{[l_i,l_{i+1}]}(l) &= l,\\
    \forall i=j+1,\ldots, N-1, \quad  
    \upsilon|_{[l_i,l_{i+1}]}(l) &= l - l_i + \hat{l}_i
    = l - l_{j+1} + \hat{l}_{j+1}.
    \end{aligned}
\end{equation}

For each coordinate function of the spline,
 (\ref{eq:miLinearSystem2}) gives a linear system $A\mathbf{M}=\mathbf{b}$
 on the second derivatives $M_i := S''(l_i)$ with 
\begin{equation}
\begin{aligned}
    \label{eq:bi}
    \forall i = 1,\ldots,N-1,\quad 
    b_i &= 6S[l_{i-1},l_i,l_{i+1}],\\
    b_0 &= {0}, \quad b_N = {0}.
\end{aligned}
\end{equation}

For each $i=0,\ldots,N-1$, 
the form of $S$ on $[l_i,l_{i+1}]$ is 
\begin{equation}
     
    \begin{array}{rl}
    \label{eq:SForm2}
\left.S\right|_{[l_i,l_{i+1}]}(l)=&
\frac{(l_{i+1} - l)^3}{6\Delta l_i} M_{i} + 
\frac{(l - l_{i})^3}{6\Delta l_i} M_{i+1} +
\left( \frac{l_{i+1} - l}{\Delta l_i} 
\right)S(l_i) + 
\left( \frac{l - l_{i}}{\Delta l_i} \right)S(l_{i+1}) \\
&- 
\frac{(\Delta l_i)^2}{6} \left[ 
\left( \frac{l_{i+1} - l}{\Delta l_i} \right)M_{i} 
+ \left( \frac{l - l_{i}}{\Delta l_i} \right)M_{i+1}
\right].
\end{array}
\end{equation}

Repeating the above processes on the perturbed knots
 yields a perturbed spline $\hat{S}$.
Denote by $\hat{M}_i:=\hat{S}''(\hat{l}_i)$
the second derivative of $\hat{S}$
and we have a new linear system
%\begin{equation*}
% \label{eq:miLinearSystemhat2}
$\hat{A}\hat{\mathbf{M}} =\hat{\mathbf{b}}$,
%\end{equation*}
where the elements $\hat{\mu}_i$, $\hat{\lambda}_i$, 
and $\hat{b}_i$ are analogous to those in
(\ref{eq:mu/lambda}) and (\ref{eq:bi}).
It follows from (\ref{eq:LhatErr})
and the direct computation
\begin{displaymath}
  \hat{\mu}_{j+1} - \mu_{j+1} =
  \frac{\hat{l}_{j+1}-\hat{l}_{j}}
  {\hat{l}_{j+2}-\hat{l}_{j}} - 
  \frac{l_{j+1}-l_{j}}{l_{j+2}-l_{j}} 
  = \frac{l_{j+1}-l_{j} + O(\epsilon)}
  {l_{j+2}-l_{j} + O(\epsilon)} - 
  \frac{l_{j+1}-l_{j}}{l_{j+2}-l_{j}} = O\left(\frac{\epsilon}{h}\right)
\end{displaymath}
% and the other terms in (\ref{eq:mu/lambdaErr}) can 
% be similarly obtained.
that $\hat{\mu}_i, \hat{\lambda}_i$ satisfy
\begin{equation}
  \label{eq:mu/lambdaErr}
  \begin{cases}
    \forall i\notin \{j-1,j,j+1\},
    & \hat{\mu}_i = \mu_i,\quad\quad\quad\quad
    \hat{\lambda}_i = \lambda_i,
    \\
    \forall i \in \{j-1, j, j+1\}, \quad
    & \hat{\mu}_i - \mu_i = O\left(\frac{\epsilon}{h}\right),
    \hat{\lambda}_i - \lambda_i = O\left(\frac{\epsilon}{h}\right).
  \end{cases}
\end{equation}
Also, (\ref{eq:bi}) gives
\begin{equation}
  \label{eq:bErr}
  \begin{cases}
    \forall i\notin \{j-1,j,j+1\},
    & \hat{b}_i = b_i,
    \\
    \forall i \in \{j-1, j, j+1\},
    &
    \hat{b}_i - b_i = 
      \mathbf{O}\left(\frac{\epsilon}{h^2}\right).
  \end{cases}
\end{equation}
Hence, 
% we could write
% \begin{equation}
%     \label{eq:hatAb}
%       \hat{A}
%      =\begin{bmatrix}
%        \lambda_1      &-1 &    \mu_1   &   &   &   &\\
%         & \ddots&   &   &   &    &\\
%         &  \hat{\mu}_{j-1}& 2 & \hat{\lambda}_{j-1} &  & &\\
%         &  &  \hat{\mu}_{j}& 2  & \hat{\lambda}_{j}  &  & \\
%         &  &  &   \hat{\mu}_{j+1}& 2  & \hat{\lambda}_{j+1}  &\\
%         &   &   &   &   & \ddots     &\\
%         &   &   &   &  \lambda_{N-1}    &-1&\mu_{N-1}
%       \end{bmatrix},\quad
%       \hat{\mathbf{b}} = 
%       \begin{bmatrix}
%         b_0 \\  \vdots \\
%         \hat{b}_{j-1} \\ \hat{b}_{j} \\ \hat{b}_{j+1}
%         \\  \vdots \\ b_{N}
%       \end{bmatrix},
% \end{equation}
% and 
for each $i=0,\ldots,N-1$,
the form of $\hat{S}$ on $[\hat{l}_i, \hat{l}_{i+1}]$ is 
\begin{equation}

\begin{array}{rl}
\label{eq:hatSForm2}
\left.\hat{S}\right|_{[\hat{l}_i,\hat{l}_{i+1}]}(\hat{l})=&
\frac{(\hat{l}_{i+1} - \hat{l})^3}{6\Delta \hat{l}_i} \hat{M}_{i} + 
\frac{(\hat{l} - \hat{l}_{i})^3}{6\Delta \hat{l}_i} \hat{M}_{i+1} +
\left( \frac{\hat{l}_{i+1} - \hat{l}}{\Delta \hat{l}_i} 
\right)\hat{S}(\hat{l}_i) + 
\left( \frac{\hat{l} - \hat{l}_{i}}{\Delta \hat{l}_i} \right)\hat{S}(\hat{l}_{i+1}) \\
&-
\frac{(\Delta \hat{l}_i)^2}{6} \left[ 
\left( \frac{\hat{l}_{i+1} - \hat{l}}{\Delta \hat{l}_i} \right)
\hat{M}_{i} + \left(
  \frac{\hat{l} - \hat{l}_{i}}{\Delta \hat{l}_i} \right)\hat{M}_{i+1}
\right].
\end{array}
\end{equation}

The two linear systems before and after the perturbation yield 
\begin{equation*}
    \begin{aligned}
    &\mathbf{b} - \hat{\mathbf{b}} = 
    A \mathbf{M} - \hat{A}\hat{\mathbf{M}} = 
    A \mathbf{M} - A \hat{\mathbf{M}} +
    A \hat{\mathbf{M}} - \hat{A}\hat{\mathbf{M}}\\
    \implies &
    A(\mathbf{M} - \hat{\mathbf{M}}) = 
     \mathbf{b} - \hat{\mathbf{b}} - 
     (A - \hat{A}) \hat{\mathbf{M}},
     \end{aligned}
\end{equation*}
which implies
\begin{equation}
\label{eq:mhatErr}
     \left\| \mathbf{M} - \hat{\mathbf{M}}\right\|_1
     \le \left\|A^{-1}\right\|_1\left(
    \left\|\mathbf{b} - \hat{\mathbf{b}} \right\|_1
    + \left\|A - \hat{A} \right\|_1
    \left\|\hat{\mathbf{M}} \right\|_1 \right)
    = O\left(\frac{\epsilon}{h^2}\right), 
\end{equation}
where the last equality follows from 
(\ref{eq:mu/lambdaErr}), (\ref{eq:bErr}), Lemma~\ref{lem:inverseA-1Norm},
and Lemma~\ref{lem:2ndDerivativeBound}.

Finally, the proof is completed by
\begin{equation*}
  
  \begin{array}{rl}
    &\int_{l_0}^{l_{j-1}} \left\|S(l) - \hat{S}
      (\upsilon(l))\right\|_2 \mathrm{d} l + 
      \int_{l_{j+1}}^{l_{N}} \left\|S(l) -
      \hat{S}(\upsilon(l)) \right\|_2 \mathrm{d} l \\
    =& \int_{l_0}^{l_{j-1}} \left\|S(l) - \hat{S}
       (l)\right\|_2 \mathrm{d} l + \int_{l_{j+1}}^{l_{N}} \left\|S(l) -
       \hat{S}(l - l_{j+1} + \hat{l}_{j+1}) \right\|_2 \mathrm{d} l\\
    =& (\sum_{i=0}^{j-2} + \sum_{i=j+1}^{N-1}) 
       \int_{l_i}^{l_{i+1}}\left\|
       \frac{(l_{i+1} - l)^3}{6\Delta l_i} (M_{i}-\hat{M}_i)
       + \frac{(l - l_{i})^3}{6\Delta l_i} (M_{i+1} - 
       \hat{M}_{i+1}) \right.\\
    &\hspace*{2.cm} -  \left.
      \frac{(\Delta l_i)^2}{6} \left[ 
      \left( \frac{l_{i+1} - l}{\Delta l_i} \right)
      (M_{i}-\hat{M}_i) 
      + \left( \frac{l - l_{i}}{\Delta l_i} \right)(M_{i+1} - 
      \hat{M}_{i+1})\right]\right\|_2 \mathrm{d} l\\
    \le& \sum_{i=0}^{N-1}
         \left( \frac{(\Delta l_i)^3}{8} \left\|M_i - \hat{M}_i\right\|_2 +
    \frac{(\Delta l_i)^3}{8} \left\|M_{i+1} - \hat{M}_{i+1}\right\|_2 \right)\\
    =& O(h^3)\cdot \sum_{i=0}^N \left\|M_i - \hat{M}_i \right\|_2
       \le O(h^3)\cdot 2\left\| \mathbf{M} - \hat{\mathbf{M}}\right\|_1
    \\
    =& O(\epsilon h),
  \end{array}
\end{equation*}
where the first step follows from 
(\ref{eq:bijectionofL}), the second from 
(\ref{eq:SForm2}) and (\ref{eq:hatSForm2}), 
% the third from the triangle inequality, 
% the fifth from the fact that $\sqrt{a^2 + b^2} < |a| + |b|$, 
and the last from (\ref{eq:mhatErr}). \qed
\end{proof}

Lemma \ref{lem:splineLocality} states that,
 over an $(r,h)$-regular sequence,
 the two cubic splines that result from
 an $O(\epsilon)$ perturbation to a breakpoint
 differ by an amount of $O(\epsilon h)$
 in the 1-norm.
% Apart from ensuring numerical stability in Lemma \ref{lem:splineStability}, 
%  Lemma \ref{lem:splineLocality} 
%  will also be useful
%  for analyzing the augmentation and adjustment errors
%  of adding and removing markers in Sec.~\ref{sec:analysis}. 
 
\begin{lem}
  \label{lem:splineStability}
  Let $\{\mathbf{X}_i\}_{i=0}^N$ be an 
  $(r, h)$-regular sequence for periodic or not-a-knot splines.
  An ${O}(\epsilon)$ perturbation to a breakpoint
  causes an $O(\epsilon)$ error to the fitted spline.
\end{lem}
\begin{proof}
  The conclusion can be proved by arguments
   similar to those in the proof of Lemma~\ref{lem:splineLocality}, 
   provided that we have $\|A^{-1} \|_\infty = O(1)$ established in
   Lemma~\ref{lem:inverseA-inftyNorm}. 
%  where $\|\cdot\|_\infty$ denotes the max-norm of a matrix.
%   For a periodic spline, the $(r, h)$-regularity of
%    the breakpoint sequence 
%    indicates that the linear system is strictly
%    diagonally dominant (by rows),
%    which implies the conclusion. 
%   In contrast, the matrix $A$ in (\ref{eq:miLinearSystem2}) 
%    for not-a-knot splines
%    is not strictly diagonally dominant,
%    in which case we define %a matrix $C$ by
%   \begin{equation}
%   \label{eq:miLinearSystem2Change}
%   C := PA, \text{ where } %\qquad
%   P
%   :=\begin{bmatrix}
%     1 & \frac{1}{2} &  &        &  &             &   \\
%     0 & 1           &  &        &  &             &   \\
%       &             &  & \ddots &  &             &   \\
%       &             &  &        &  & 1           & 0 \\
%       &             &  &        &  & \frac{1}{2} & 1
%   \end{bmatrix}.
%   \end{equation}
%   Then, for the first row of $C$, we have 
% %  \begin{equation*}
%     $|c_{1, 1} | = \lambda_1 + \frac{1}{2}\mu_1 
%     > \mu_1 + \frac{1}{2}\lambda_1 
%     = \sum_{j=2}^{n} |c_{1, j} |$
% %  \end{equation*}
%   where the inequality follows from $\lambda_1 > \mu_1$ in 
%    (\ref{eq:mu1/geq/lambda1}). 
%   Similarly, 
%   we can verify the condition for the last row, which 
%    implies that $C$ is strictly diagonally dominant %by rows 
%    and $\|C^{-1} \|_\infty = O(1)$.
%   Hence, $\|A^{-1} \|_\infty 
%    \leq \|C^{-1} \|_\infty \|P \|_\infty = O(1)$.  
   \qed
\end{proof}

%%% Local Variables:
%%% mode: latex
%%% TeX-master: "../MARS-n2D"
%%% End:
